# Supplementary material for: First Extraction of Transverse Momentum Dependent Helicity Distributions
Source: arXiv:2409.08110 source file (2025-03-31)
Supplement: Supplementary file 1 [file supplemental_material.pdf]

# Supplementary Material: First Extraction of Transverse Momentum Dependent Helicity Distributions

Ke Yang,[1] Tianbo Liu,[2,3,*] Peng Sun,[4,5,†] Yuxiang Zhao,[3,4,5,6,‡] and Bo-Qiang Ma[1,7,8,§]
(Transverse Nucleon Tomography Collaboration)
[1]*School of Physics, Peking University, Beijing 100871, China*
[2]*Key Laboratory of Particle Physics and Particle Irradiation (MOE), Institute of Frontier and Interdisciplinary Science, Shandong University, Qingdao, Shandong 266237, China*
[3]*Southern Center for Nuclear-Science Theory (SCNT), Institute of Modern Physics, Chinese Academy of Sciences, Huizhou 516000, China*
[4]*Institute of Modern Physics, Chinese Academy of Sciences, Lanzhou, Gansu Province 730000, China*
[5]*University of Chinese Academy of Sciences, Beijing 100049, China*
[6]*Key Laboratory of Quark and Lepton Physics (MOE) and Institute of Particle Physics, Central China Normal University, Wuhan 430079, China*
[7]*Center for High Energy Physics, Peking University, Beijing 100871, China*
[8]*School of Physics, Zhengzhou University, Zhengzhou 450001, China*

## I. THE RESULTS OF PARAMETERS

The fitted results of the parameters are summarized in Table I (this document), where the central values are evaluated from the average of the 1000 replicas, and the upper and lower uncertainties represent the standard deviation from the central values on each side. The correlation matrix among the parameters are provided in Table II (this document). A visualization of the correlation matrix is in Fig. 1 (this document).

## II. COMPARISON WITH EXPERIMENTAL MEASUREMENTS

The comparisons between experimental data and our fit results are shown in Figs. 2 to 11 (this document), in which the filled points represent the data included in the fit and the open points represent those excluded from the fit due to the cut $P_{hT}/(zQ) < 0.5$. The term "CSA" refers to the cross-section asymmetry, indicating that these measurements contain the kinematic factors.

TABLE I. Central values and uncertainties of the parameters from the fit.

| Parameter | Value | Parameter | Value |
|---|---|---|---|
| $N_u$ | $0.0223^{+0.0029}_{-0.0024}$ | $N_{\bar{u}}$ | $-0.008^{+0.092}_{-0.035}$ |
| $N_d$ | $0.0353^{+0.0051}_{-0.0088}$ | $N_{\bar{d}}$ | $0.006^{+0.032}_{-0.011}$ |
| $N_s$ | $-0.022^{+0.043}_{-0.043}$ | $N_g$ | $0.0220^{+0.0081}_{-0.0706}$ |
| $\alpha_u$ | $2.78^{+0.45}_{-0.72}$ | $\alpha_d$ | $4.28^{+0.38}_{-0.76}$ |
| $\beta_u$ | $0.145^{+0.041}_{-0.194}$ | $\beta_d$ | $1.16^{+0.14}_{-0.40}$ |
| $\epsilon_u$ | $7.4^{+2.3}_{-4.5}$ | $\epsilon_d$ | $-0.59^{+0.18}_{-0.20}$ |
| $\lambda_1$ | $0.240^{+0.062}_{-0.134}$ | $\lambda_2$ | $0.39^{+0.13}_{-0.33}$ |
| $\lambda_3$ | $0.92^{+12.17}_{-0.92}$ | $\lambda_4$ | $7.50^{+2.29}_{-0.78}$ |
| $\lambda_5$ | $-1.11^{+0.87}_{-0.50}$ | | |

* liutb@sdu.edu.cn
† pengsun@impcas.ac.cn
‡ yxzhao@impcas.ac.cn
§ mabq@pku.edu.cn

TABLE II. Correlations among various parameters.

| | $N_u$ | $N_d$ | $N_s$ | $N_{\bar{u}}$ | $N_{\bar{d}}$ | $N_g$ | $\alpha_u$ | $\alpha_d$ | $\beta_u$ | $\beta_d$ | $\epsilon_u$ | $\epsilon_d$ | $\lambda_1$ | $\lambda_2$ | $\lambda_3$ | $\lambda_4$ | $\lambda_5$ |
|---|---|---|---|---|---|---|---|---|---|---|---|---|---|---|---|---|---|
| $N_u$ | 1 | 0.540 | 0.071 | −0.155 | 0.006 | −0.058 | −0.101 | −0.089 | −0.127 | −0.125 | −0.048 | −0.066 | 0.064 | 0.128 | −0.006 | 0.025 | 0.005 |
| $N_d$ | 0.540 | 1 | −0.160 | −0.156 | −0.178 | −0.053 | 0.340 | −0.097 | 0.224 | 0.229 | −0.003 | 0.084 | 0.292 | −0.112 | 0.013 | 0.046 | 0.021 |
| $N_s$ | 0.071 | −0.160 | 1 | 0.164 | −0.037 | 0.039 | −0.132 | −0.006 | −0.156 | −0.099 | −0.160 | −0.037 | −0.126 | 0.075 | −0.028 | −0.053 | −0.002 |
| $N_{\bar{u}}$ | −0.155 | −0.156 | 0.164 | 1 | 0.623 | −0.062 | −0.157 | −0.090 | −0.141 | −0.196 | −0.062 | −0.046 | −0.062 | 0.110 | 0.019 | −0.019 | 0.095 |
| $N_{\bar{d}}$ | 0.006 | −0.178 | −0.037 | 0.623 | 1 | −0.009 | −0.077 | −0.080 | −0.103 | −0.095 | −0.045 | 0.079 | −0.036 | 0.077 | 0.029 | −0.023 | 0.084 |
| $N_g$ | −0.058 | −0.053 | 0.039 | −0.062 | −0.009 | 1 | 0.023 | −0.105 | −0.025 | −0.099 | 0.070 | 0.080 | 0.087 | 0.093 | 0.013 | 0.020 | 0.008 |
| $\alpha_u$ | −0.101 | 0.340 | −0.132 | −0.157 | −0.077 | 0.023 | 1 | 0.411 | 0.682 | 0.510 | 0.047 | −0.066 | 0.257 | −0.266 | 0.016 | 0.009 | 0.039 |
| $\alpha_d$ | −0.089 | −0.097 | −0.006 | −0.090 | −0.080 | −0.105 | 0.411 | 1 | 0.310 | 0.514 | −0.027 | −0.047 | 0.060 | −0.063 | 0.010 | 0.008 | −0.042 |
| $\beta_u$ | −0.127 | 0.224 | −0.156 | −0.141 | −0.103 | −0.025 | 0.682 | 0.310 | 1 | 0.670 | −0.044 | −0.008 | 0.021 | −0.324 | 0.006 | 0.018 | 0.029 |
| $\beta_d$ | −0.125 | 0.229 | −0.099 | −0.196 | −0.095 | −0.099 | 0.510 | 0.514 | 0.670 | 1 | 0.027 | −0.001 | 0.104 | −0.246 | −0.003 | 0.027 | −0.002 |
| $\epsilon_u$ | −0.048 | −0.003 | −0.160 | −0.062 | −0.045 | 0.070 | 0.047 | −0.027 | −0.044 | 0.027 | 1 | 0.072 | 0.026 | 0.008 | −0.018 | 0.019 | 0.009 |
| $\epsilon_d$ | −0.066 | 0.084 | −0.037 | −0.046 | 0.079 | 0.080 | −0.066 | −0.047 | −0.008 | −0.001 | 0.072 | 1 | 0.065 | −0.005 | −0.009 | −0.007 | −0.006 |
| $\lambda_1$ | 0.064 | 0.292 | −0.126 | −0.062 | −0.036 | 0.087 | 0.257 | 0.060 | 0.021 | 0.104 | 0.026 | 0.065 | 1 | 0.143 | 0.021 | 0.037 | 0.262 |
| $\lambda_2$ | 0.128 | −0.112 | 0.075 | 0.110 | 0.077 | 0.093 | −0.266 | −0.063 | −0.324 | −0.246 | 0.008 | −0.005 | 0.143 | 1 | −0.003 | −0.004 | −0.129 |
| $\lambda_3$ | −0.006 | 0.013 | −0.028 | 0.019 | 0.029 | 0.013 | 0.016 | 0.010 | 0.006 | −0.003 | −0.018 | −0.009 | 0.021 | −0.003 | 1 | 0.002 | −0.001 |
| $\lambda_4$ | 0.025 | 0.046 | −0.053 | −0.019 | −0.023 | 0.020 | 0.009 | 0.008 | 0.018 | 0.027 | 0.019 | −0.007 | 0.037 | −0.004 | 0.002 | 1 | −0.001 |
| $\lambda_5$ | 0.005 | 0.021 | −0.002 | 0.095 | 0.084 | 0.008 | 0.039 | −0.042 | 0.029 | −0.002 | 0.009 | −0.006 | 0.262 | −0.129 | −0.001 | −0.001 | 1 |

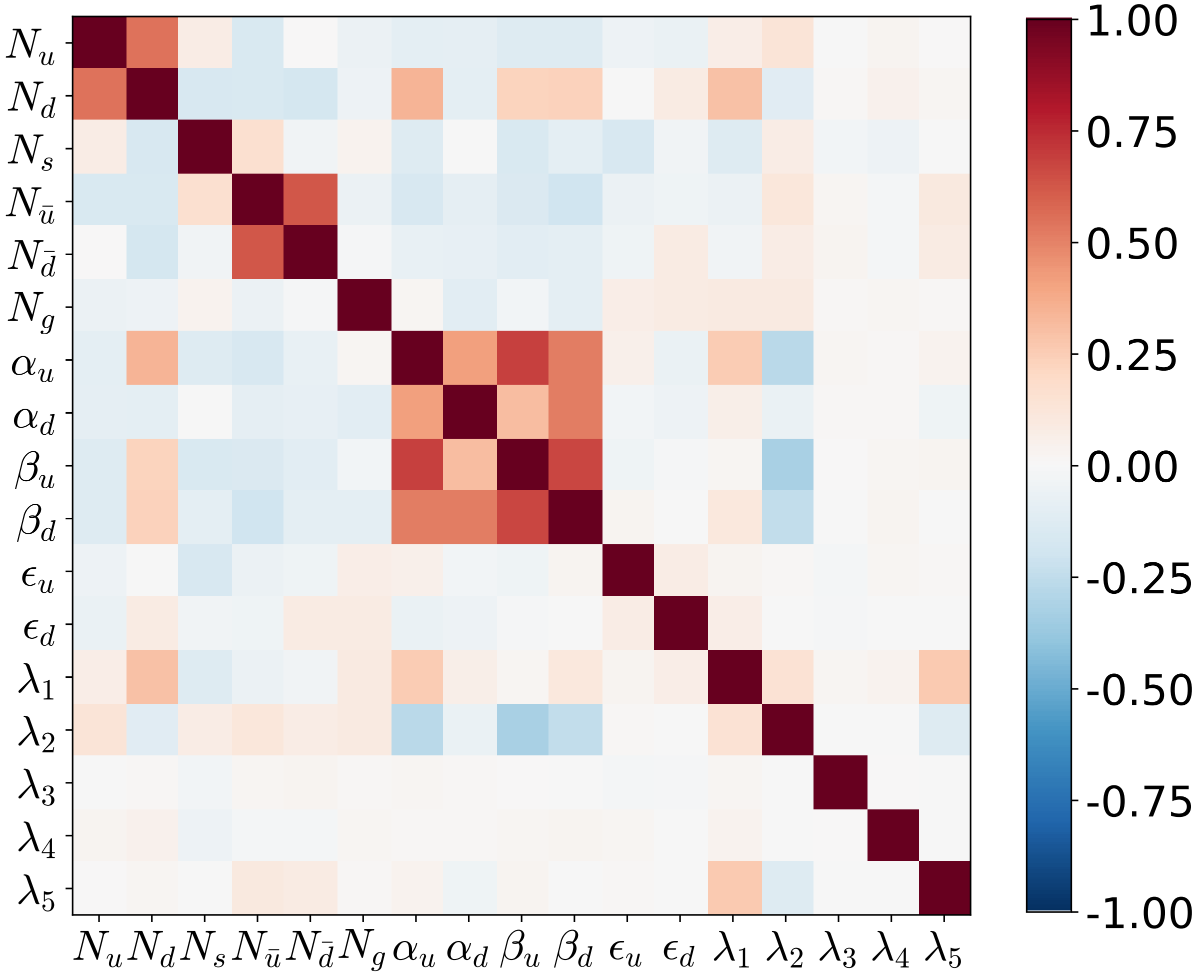


FIG. 1. A visualization of the correlation matrix of the parameters.

TABLE III. The correlated relative uncertainties provided by each experimental data set.

| Experiment | Process | Data points | Beam and target polarization | Dilution |
|---|---|---|---|---|
| HERMES[1] | $e^{\pm}p \to e^{\pm}hX$ | 84 (160) | 6.6% | 0 |
| HERMES[1] | $e^{\pm}d \to e^{\pm}hX$ | 160 (317) | 5.7% | 1.7% |
| CLAS[2] | $e^{-}p \to e^{-}\pi^0 X$ | 9 (21) | 4.5% | 5.8% |
| Total | | 253 (498) | | |

## III. CORRELATED UNCERTAINTIES OF THE EXPERIMENTAL DATA

We summarized the correlated relative uncertainties of each experimental data set in Table III (this document), which are provided in corresponding publications [1, 2].

## IV. THE POSITIVITY BOUND

According to the probability interpretations of TMD PDFs, one can obtain the positivity bound $|g_{1L}| \leq f_1$, which is not imposed during the fitting. Instead, we examine the positivity bound below by comparing the extracted $g_{1L}(x, b)$

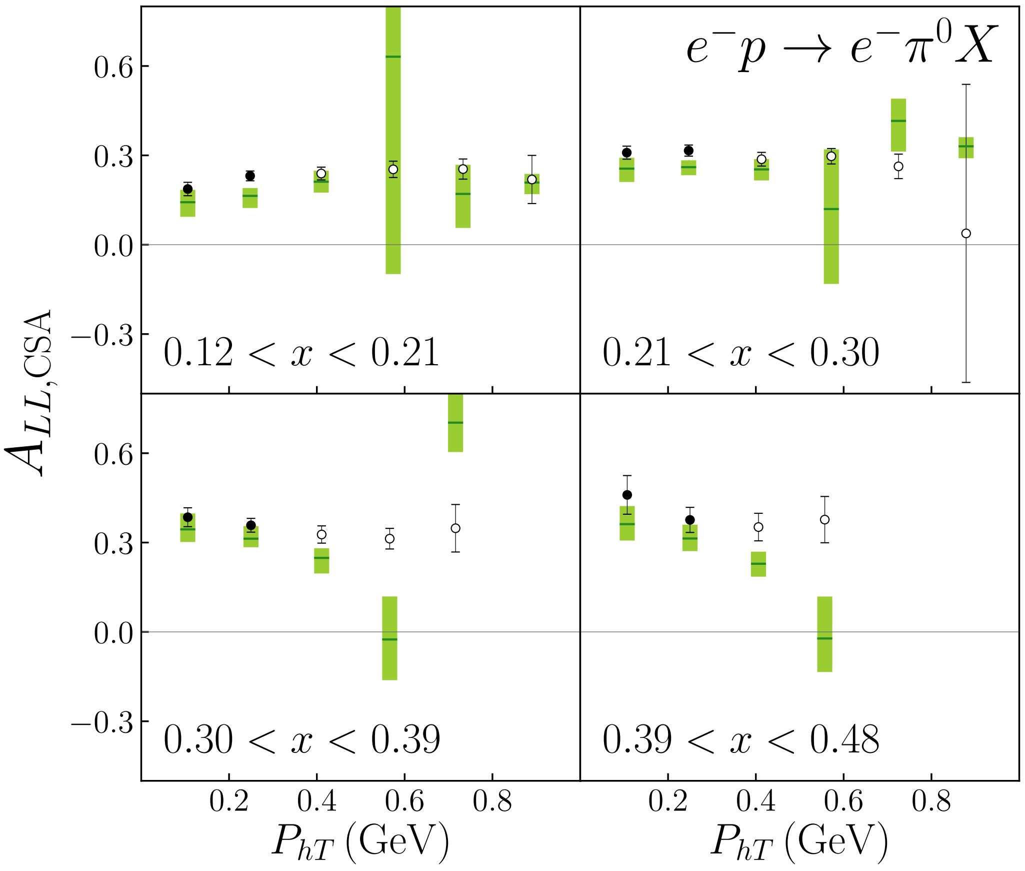


FIG. 2. Comparison between our results and CLAS data [2].

with the unpolarized distribution $f_1(x, b)$ in Fig. 12 (this document). Considering the uncertainties, one can find that the positivity is not violated.

## V. RESULT FROM FIT USING COLLINEAR HELICITY DISTRIBUTION AS INPUT

As mentioned in the main text, we adopt a flexible $x$-dependent parametrization. For comparison, we also perform the analysis with fixed $x$-shape as collinear helicity distributions by setting $\alpha = \beta = \epsilon = 0$ in Eq. (17) (main text). The comparison between results with fixed $x$-shape and those with flexible $x$-dependent parametrization as our main results is shown in Fig. 13. They are consistent with each other according to the uncertainties.

[1] A. Airapetian *et al.* (HERMES Collaboration), Longitudinal double-spin asymmetries in semi-inclusive deep-inelastic scattering of electrons and positrons by protons and deuterons, Phys. Rev. D **99**, no.11, 112001 (2019).

[2] S. Jawalkar *et al.* (CLAS Collaboration), Semi-Inclusive $\pi_0$ target and beam-target asymmetries from 6 GeV electron scattering with CLAS, Phys. Lett. B **782**, 662 (2018).

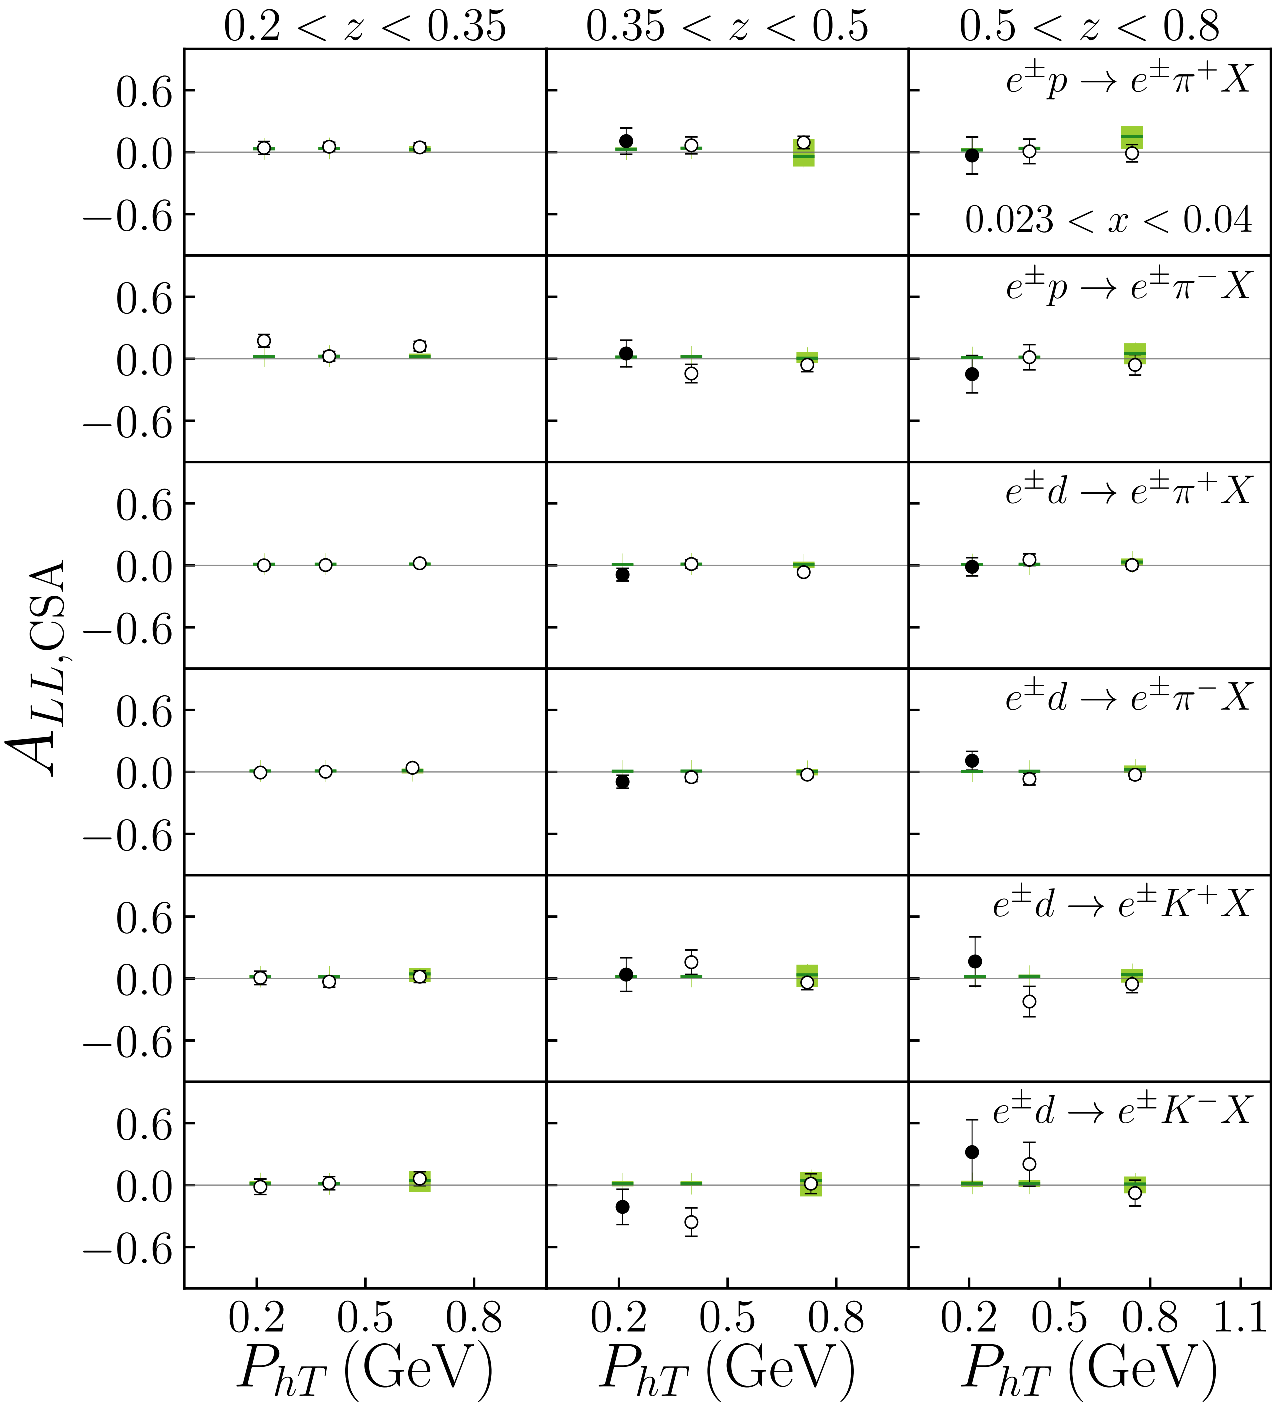


FIG. 3. Comparison between our results and HERMES data [1].

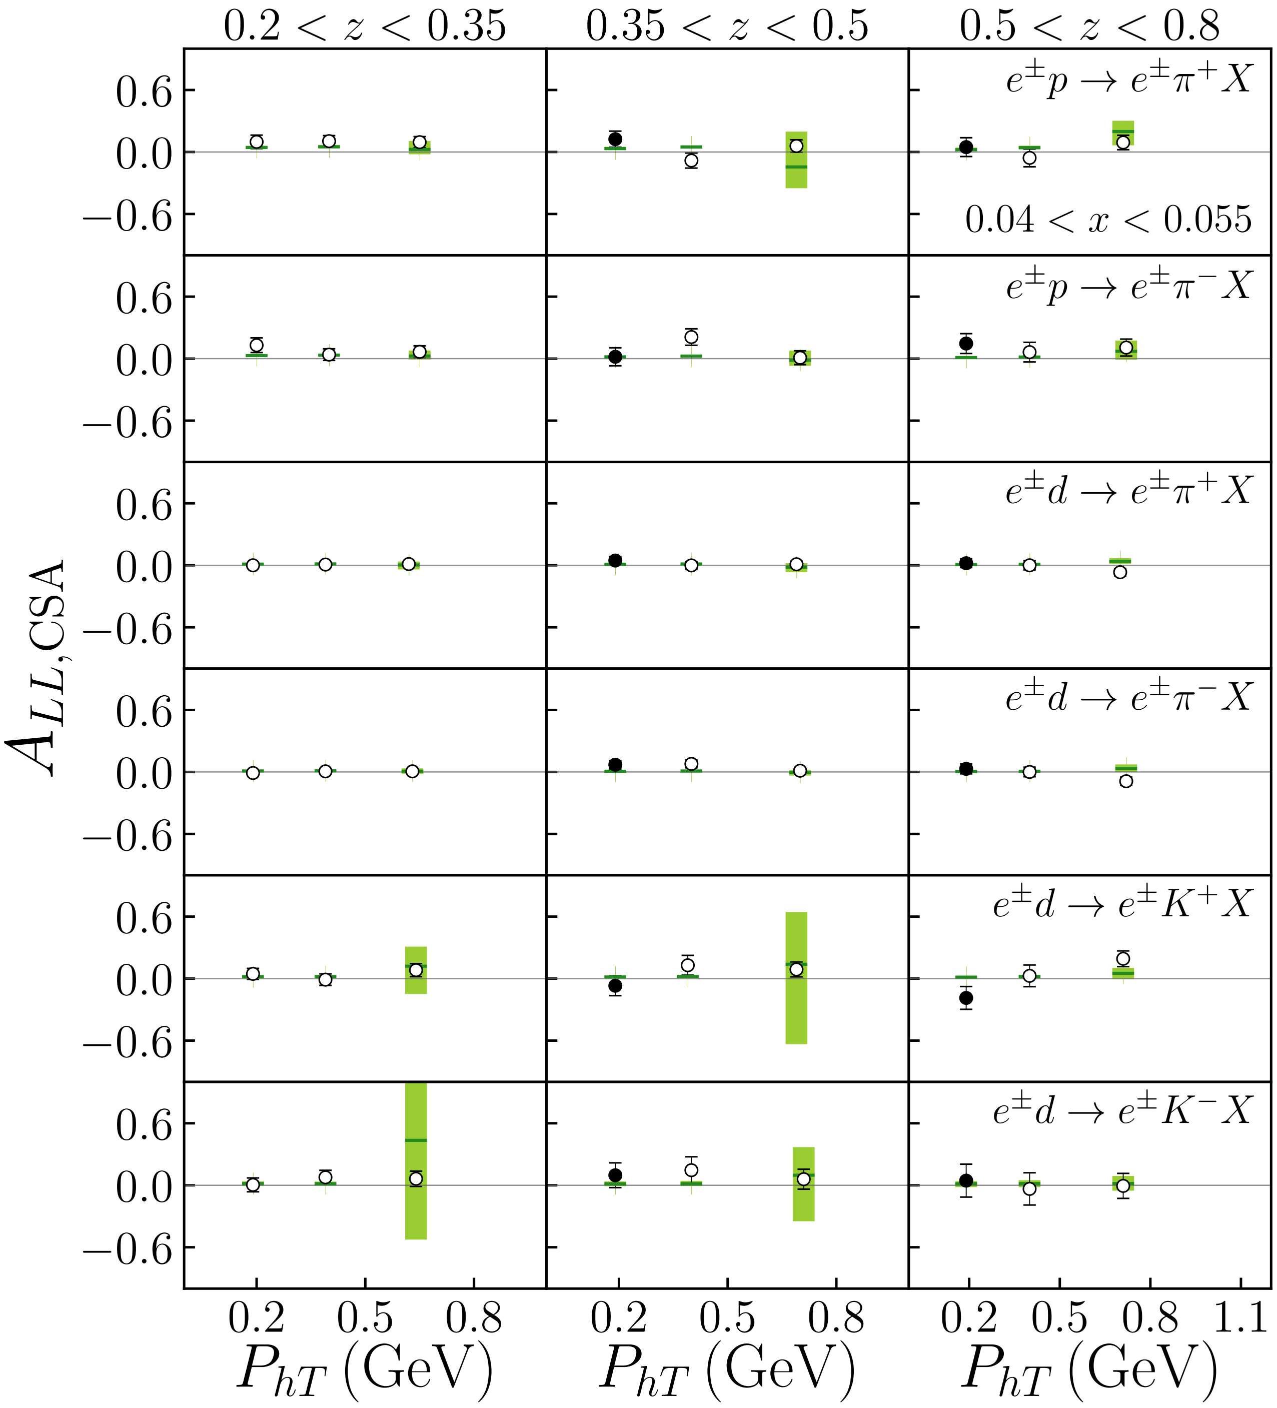


FIG. 4. Comparison between our results and HERMES data [1].

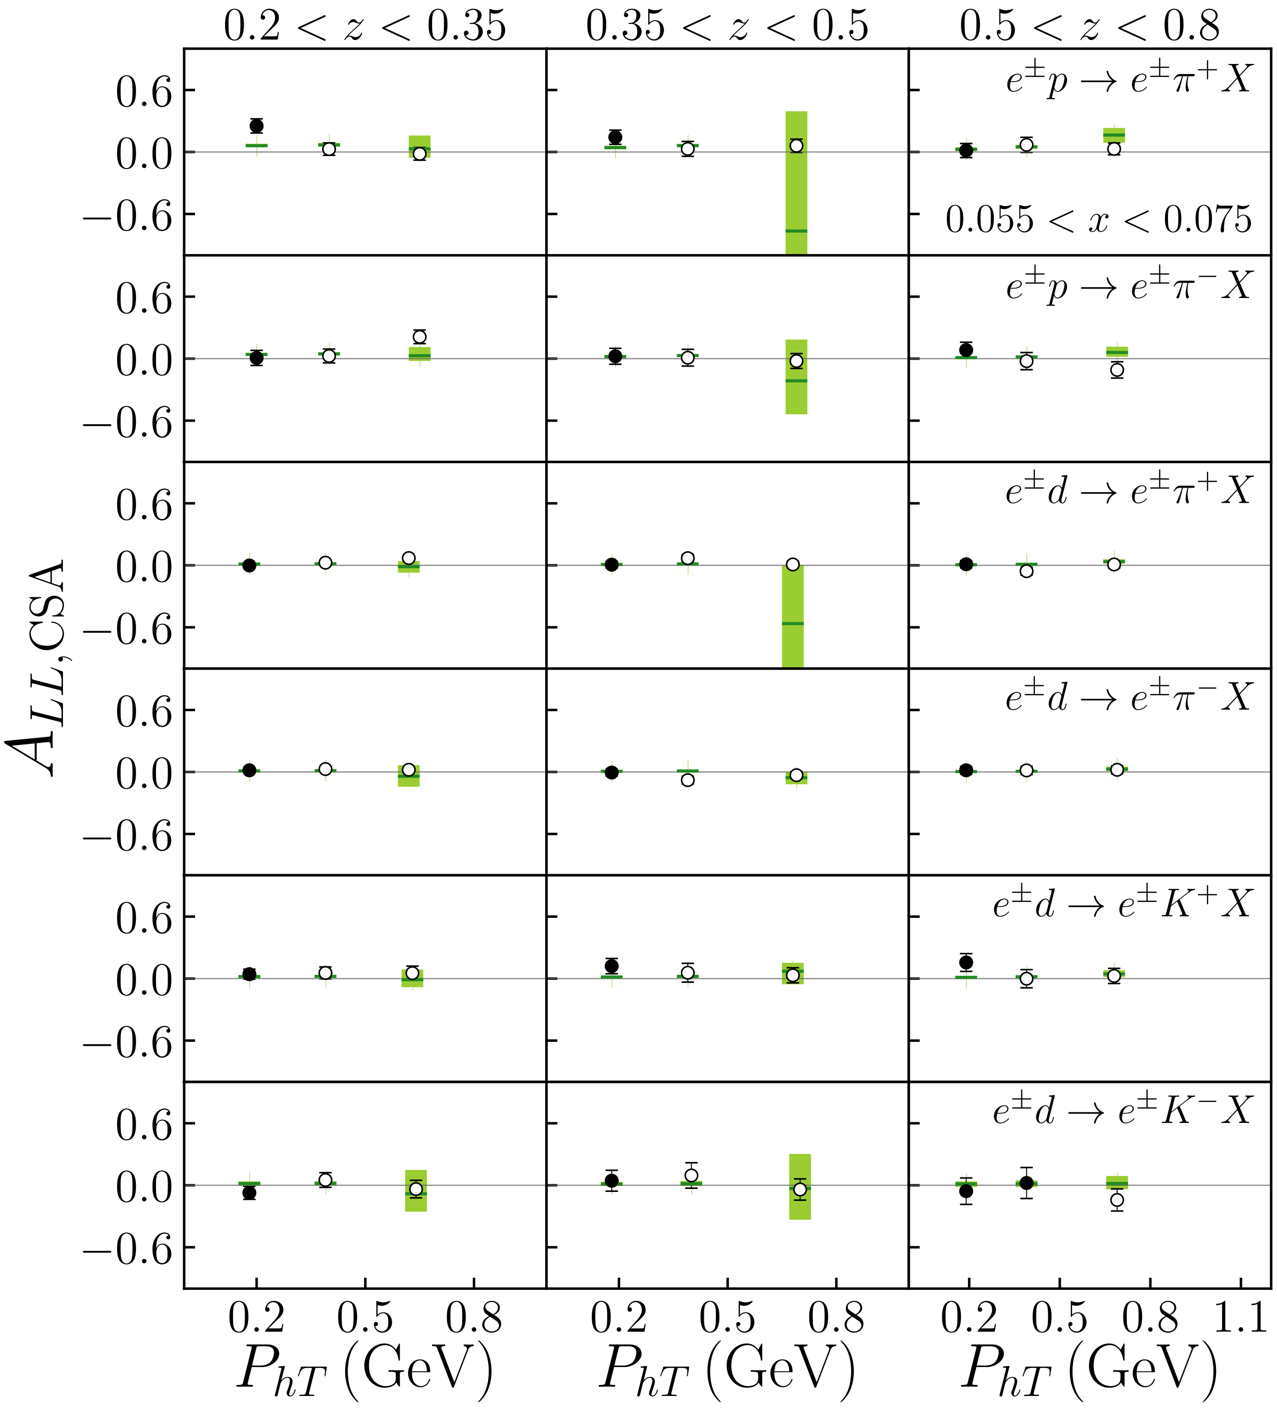


FIG. 5. Comparison between our results and HERMES data [1].

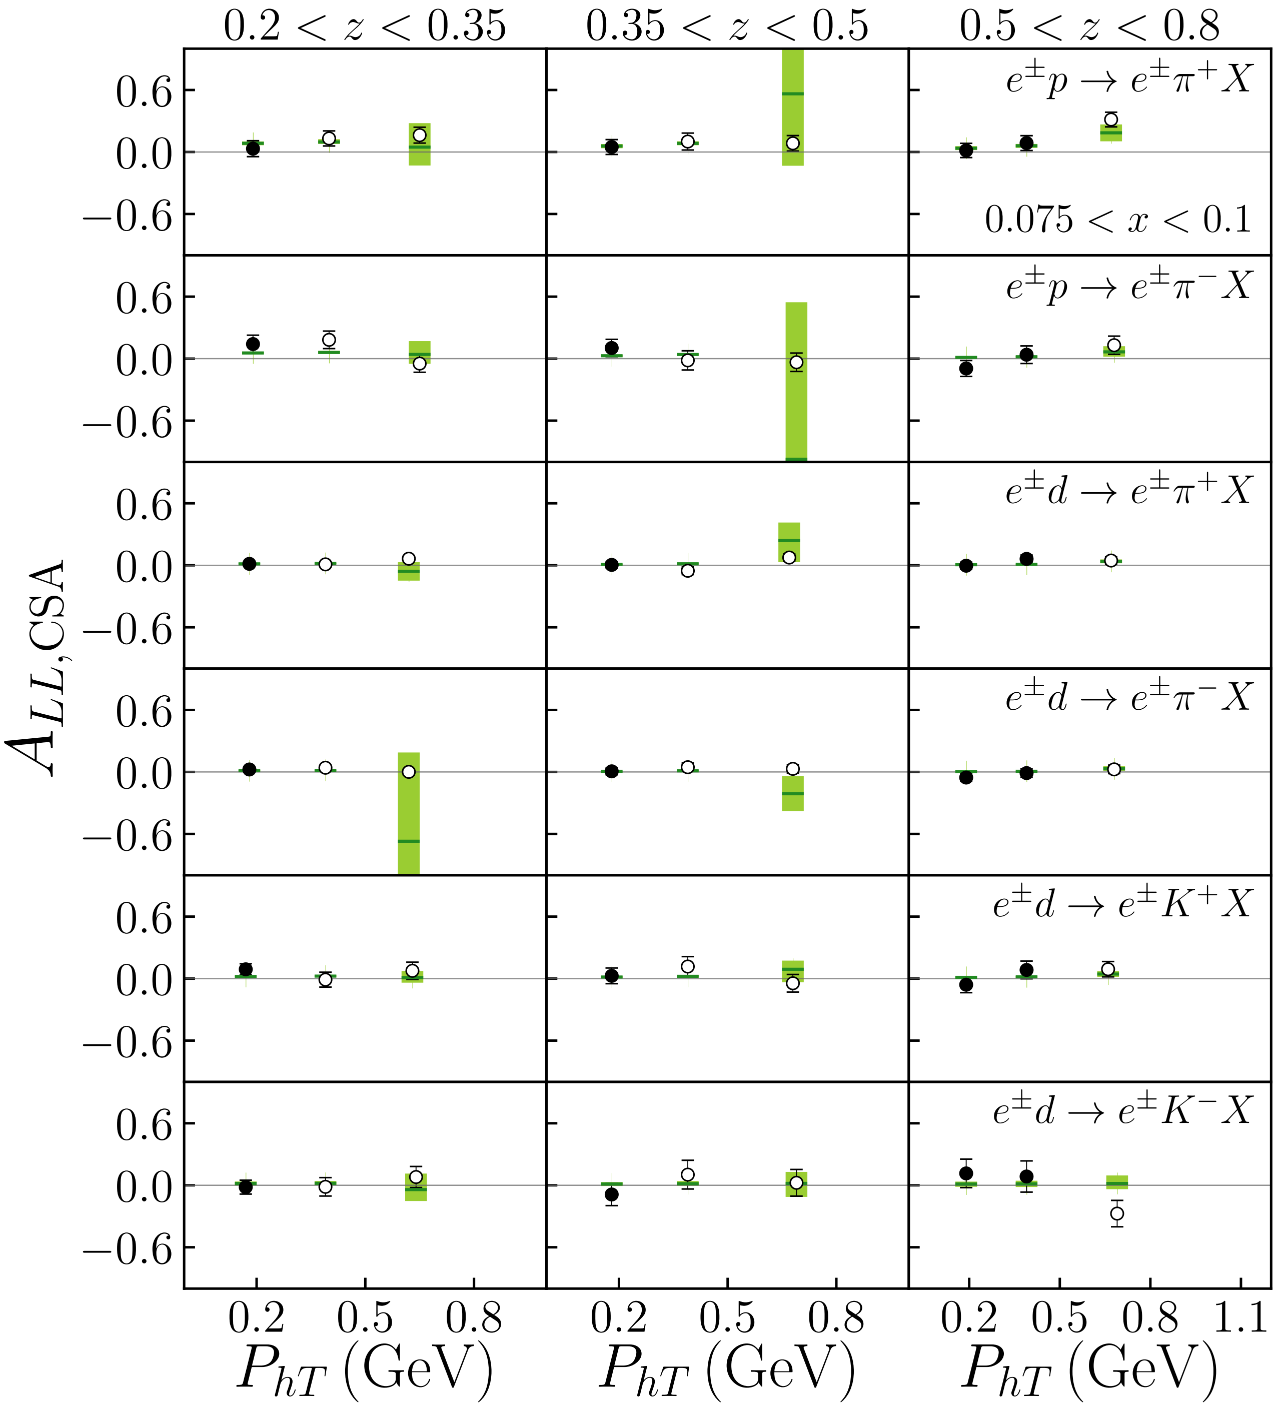


FIG. 6. Comparison between our results and HERMES data [1].

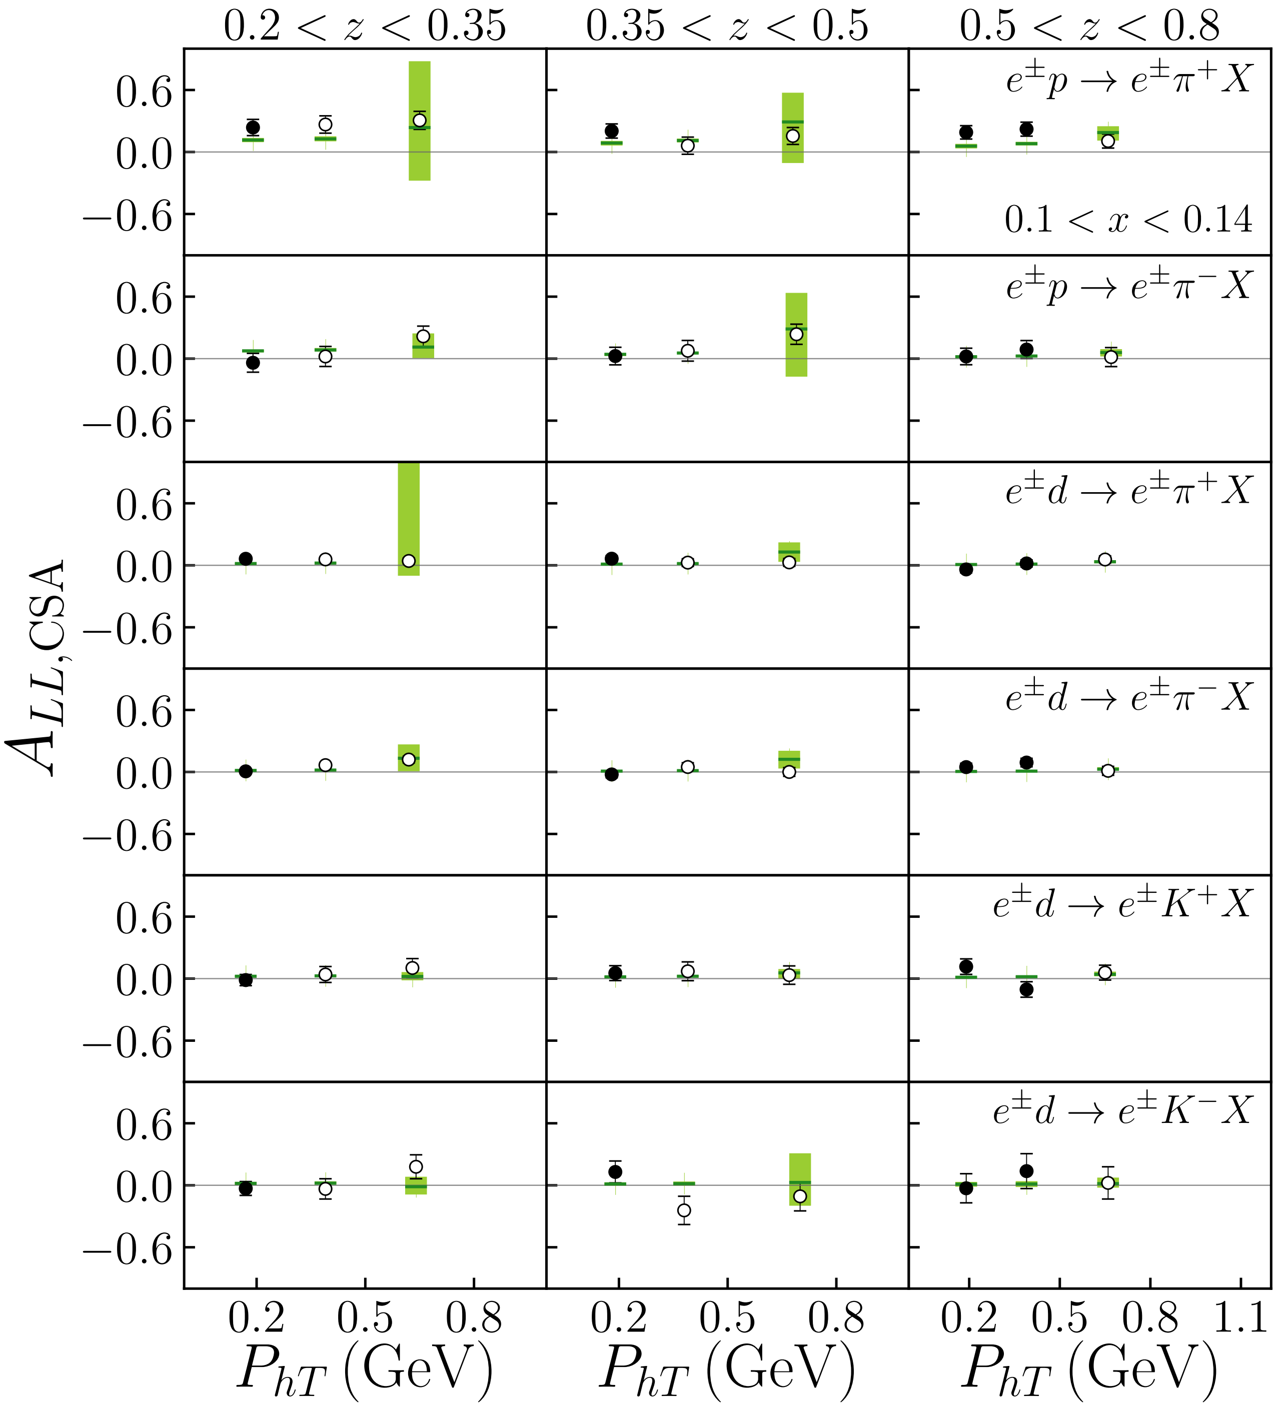


FIG. 7. Comparison between our results and HERMES data [1].

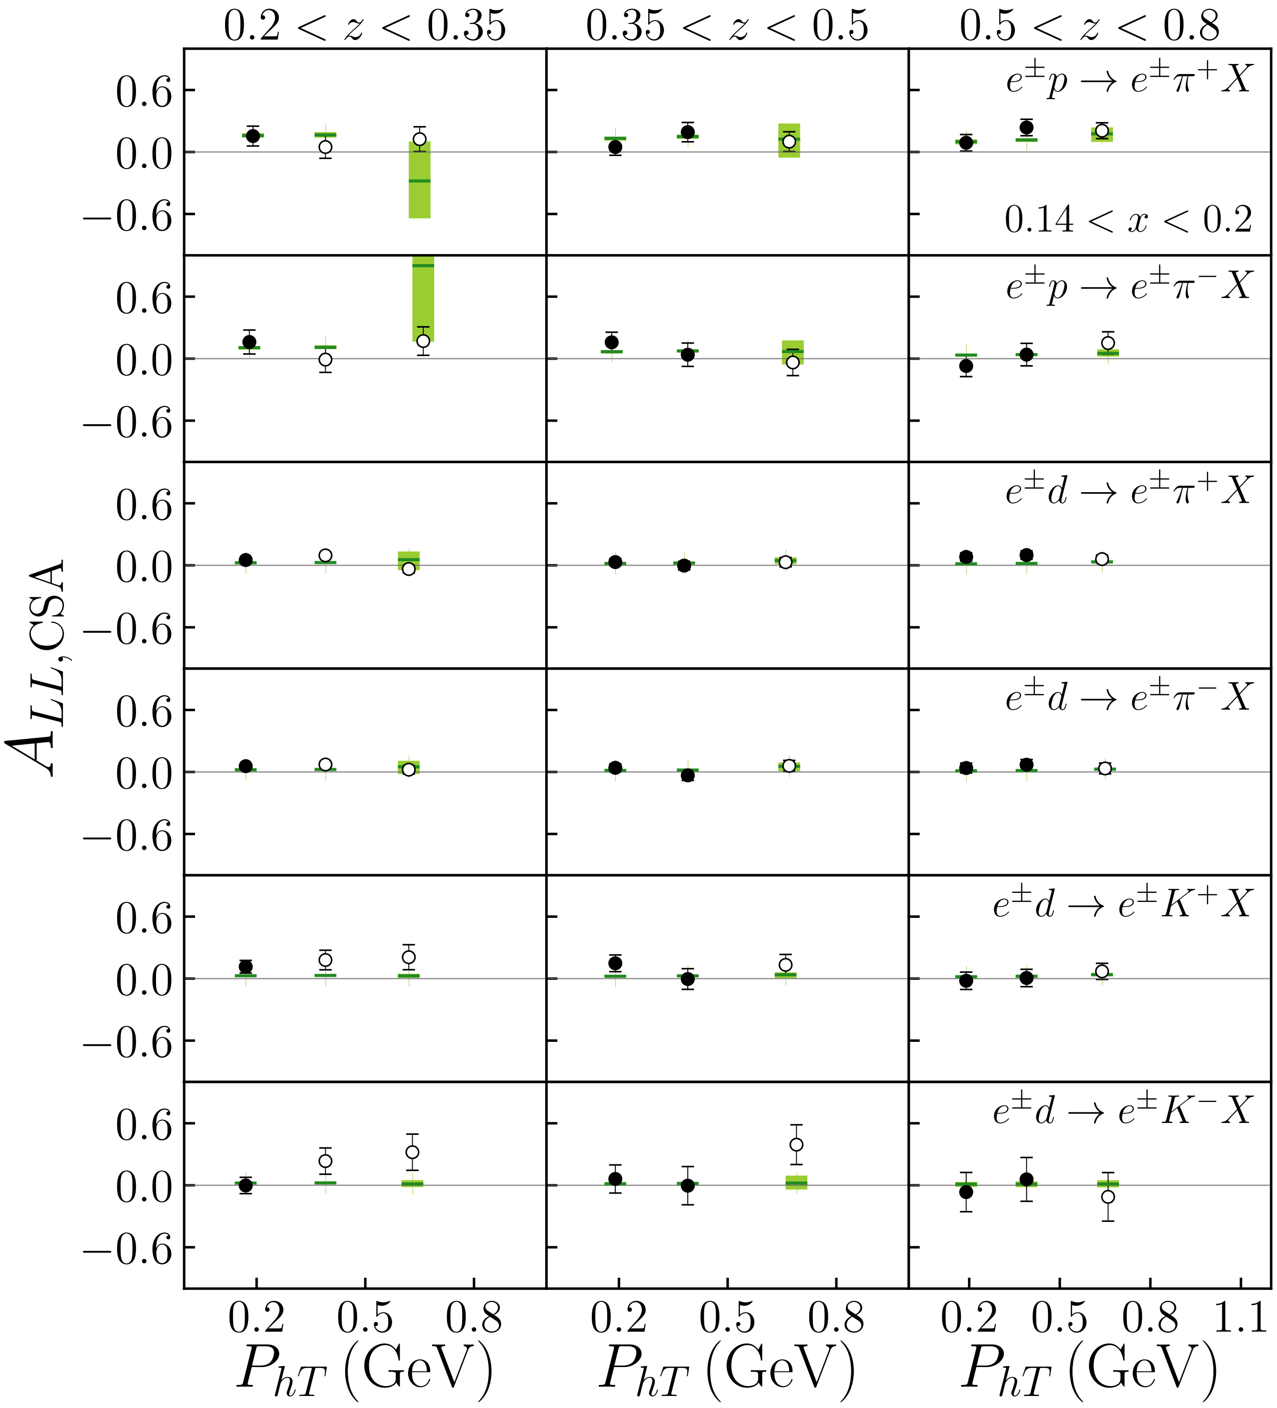


FIG. 8. Comparison between our results and HERMES data [1].

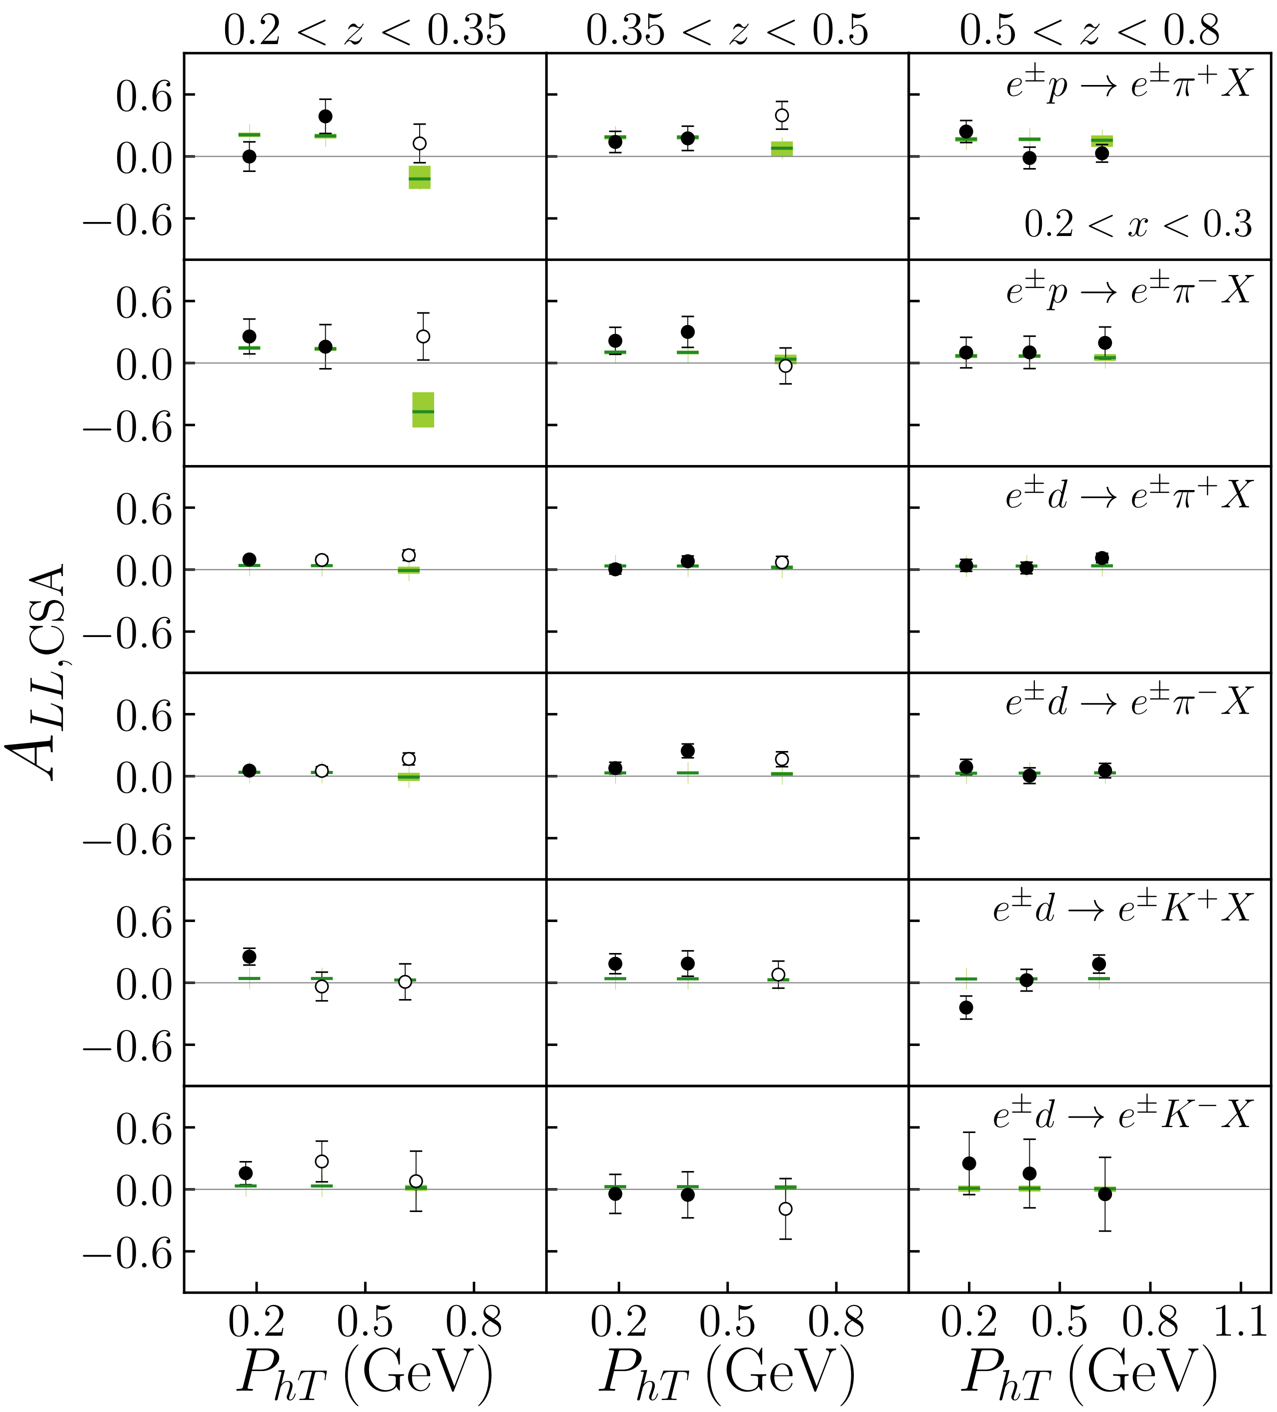


FIG. 9. Comparison between our results and HERMES data [1].

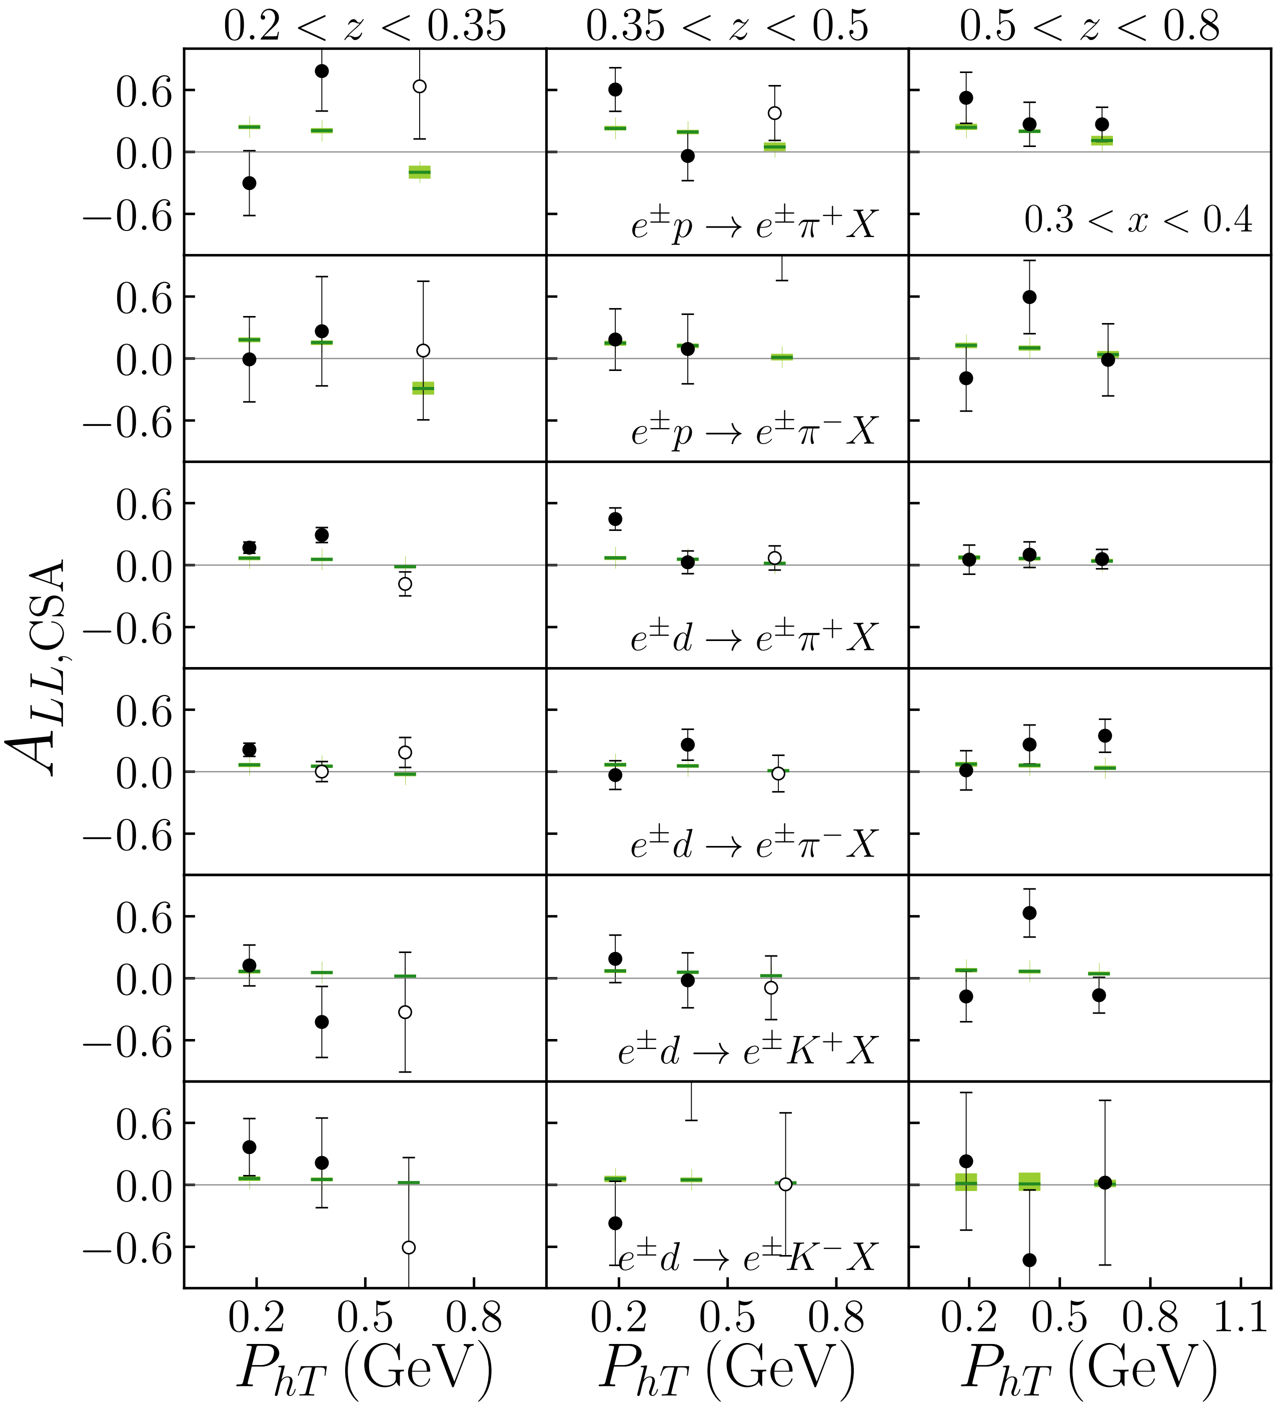


FIG. 10. Comparison between our results and HERMES data [1].

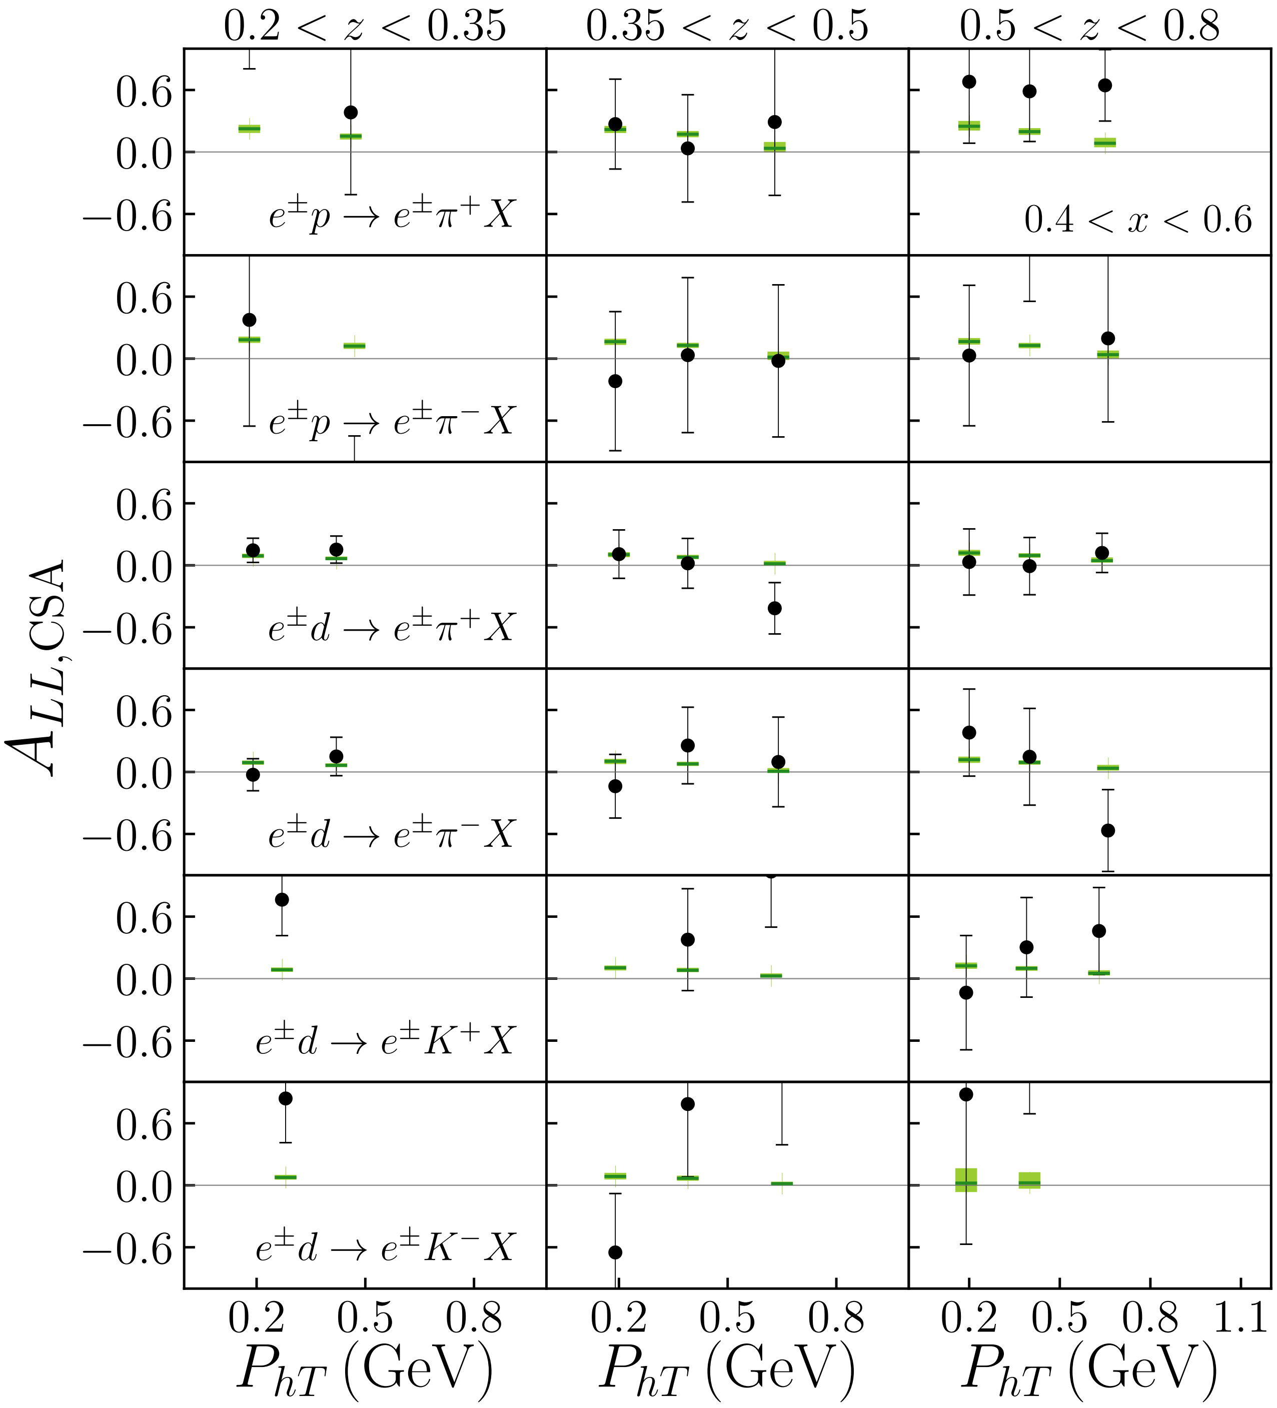


FIG. 11. Comparison between our results and HERMES data [1].

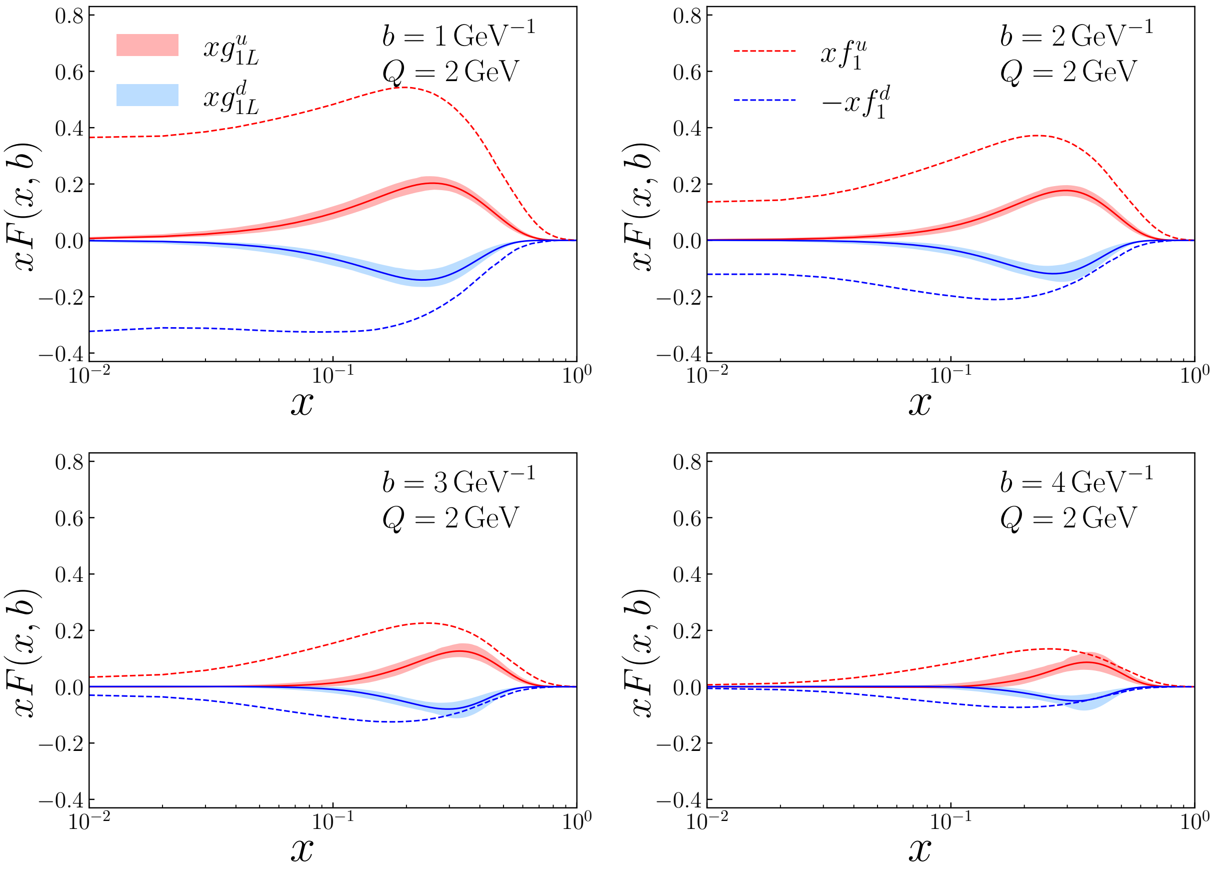


FIG. 12. Comparison between our extracted $xg_{1L}(x, b)$ and the unpolarized distributions $xf_1(x, b)$ in SV19 fit. Here $F = g_{1L}^u, g_{1L}^d, f_1^u, -f_1^d$. The solid curves with bands represent the central values and $1\sigma$ uncertainties of the helicity distributions $xg_{1L}^{u,d}(x, b)$. The dashed curves represent the unpolarized distributions $xf_1^{u,d}(x, b)$ from SV19 fit.

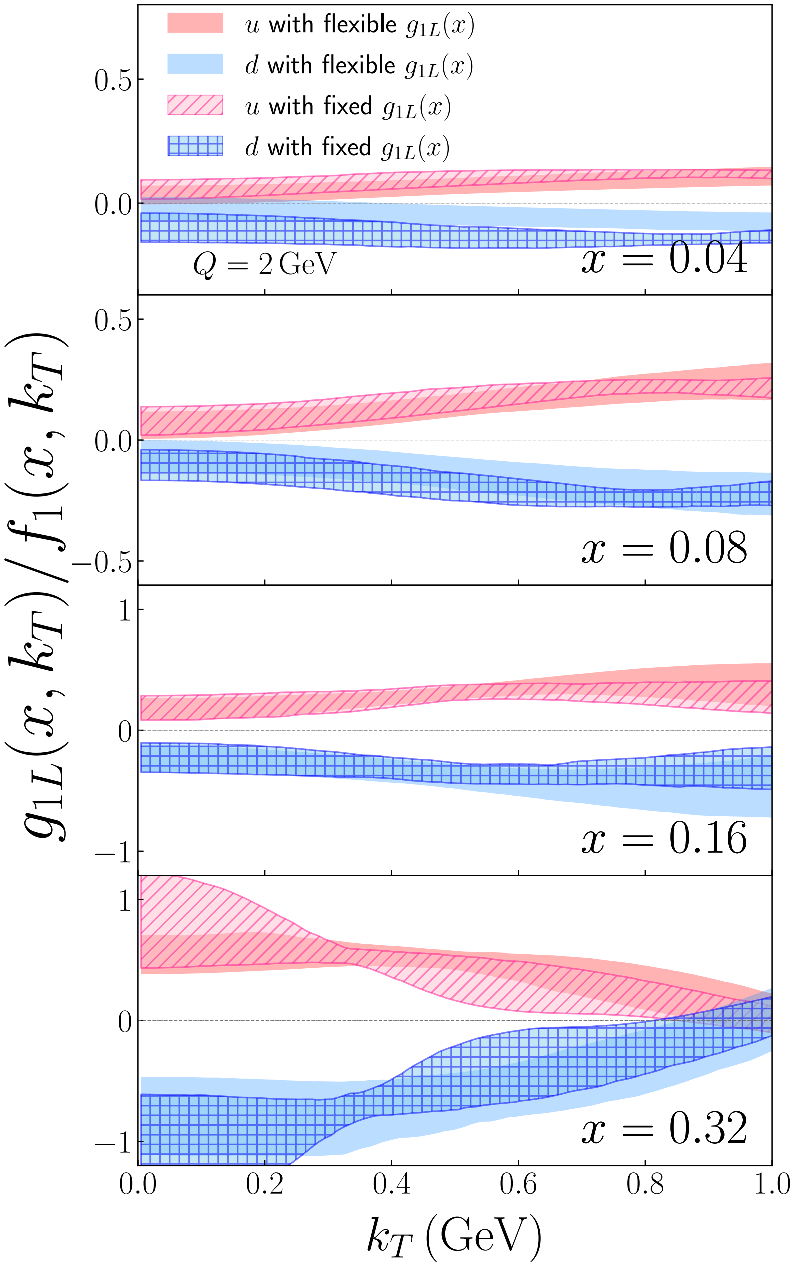


FIG. 13. Comparison between extracted polarization distributions with fixed $x$-shape and flexible $x$-shape parametrizations.
